# Supplementary material for: Efficiently Hardening SGX Enclaves against Memory Access Pattern Attacks via Dynamic Program Partitioning
Source: arXiv:2212.12656 source file (2022-12-27)
Supplement: Supplementary file 1 [file wellformated_appendix.tex]

\vspace{0.2in}
\noindent{}{\LARGE \bf Appendix}

\section{Further Comparison with Existing Methods}
\label{sec:approach}
Our method for engineering external obliviousness is that given the target computation expressed by an external-oblivious algorithm, we place and only place the part of the program accessing internal memory in external-oblivious algorithms to the HTM transactions. By this means, the cache-misses which only occur between transactions are oblivious, while cache-hits and other internal accesses can be made secure by HTM protection.

The motivation to combine HTM and external oblivious algorithms can be better illustrated by an example: Consider implementing a sort on Intel SGX with cache-attack security. The first baseline (BL1) entails implementing the word-oblivious sorting network at the expense of a logarithmic multiplicative factor (i.e., $O(N\log^2{N})$). The second baseline is to use HTM to protect the leaky accesses in a classic sorting algorithm of $O(N\log{N})$ complexity, such as quicksort or merge sort. This approach limits the data size by CPU cache size. In a big-data setting (with large $N$), neither approach is feasible as the former is inefficient and the latter is unscalable. By contrast, our proposed method combining HTM and external oblivious algorithms could lead to an optimal $O(N\log{N})$ sorting algorithm (based on the scramble-then-shuffle paradigm~\cite{DBLP:journals/popets/DangDCO17}) implemented with cache-attack security.

Note that our approach shares some general ideas with Cloak and T-SGX in the sense that it leverages Intel TSX to detect memory-access attacks. However, Cloak does not automatically partition the computation and is limited to the small-data case. T-SGX is a static program-partition scheme, which limits its applicability in handling loops and thus big-data computations. Our work uniquely addresses the problem of dynamically partitioning the programs to support big-data computations with access-pattern security.
